# Supplementary material for: ROSTrans: Empirically Benchmarking LLMs for ROS1-to-ROS2 Migration
Source: arXiv:2610.41168 source file (2026-10-30)
Supplement: Supplementary file 1 [file 9-Appendix.tex]

\section{Sensitivity Analysis of RWS Weights}
\label{appdx:a}
To evaluate the empirical robustness of the Risk Weighted Score (RWS) and to ensure that the benchmark conclusions are not overly sensitive to the subjective assignment of error category weights, we perform a comprehensive sensitivity analysis. We examine three distinct weight configurations that reflect alternative evaluation priorities and risk tolerances:

\begin{itemize}[leftmargin=*]
    \item \textbf{Original (Baseline):} The default weight assignment utilized in the main text ($w_A=0.5, w_B=0.2, w_C=0.1, w_{E2}=0.05$), which is calibrated based on domain expertise and robotic safety considerations.
    \item \textbf{Linear:} A configuration characterized by a gradual, linear decay of weights across the hierarchy ($w_A=0.4, w_B=0.3, w_C=0.2, w_{E2}=0.1$), thereby reducing the mathematical disparity between high-risk and low-risk defect categories.
    \item \textbf{Strict\_E2:} A configuration that imposes an exceptionally stringent penalty on covert risks ($w_{E2}=0.01$) while maintaining high penalties for other categories ($w_A=0.8, w_B=0.4, w_C=0.1$), simulating a deployment scenario with near-zero tolerance for hidden behavioral failures.
\end{itemize}

\begin{figure}[htbp]
    \centering
    \includegraphics[width=\textwidth]{figures/01_RWS_Sensitivity_Analysis_1x3.pdf}
    \caption{Sensitivity analysis of LLM performance rankings under three distinct RWS weight configurations (Original, Linear, and Strict\_E2). The models across all subplots are ordered consistently according to the baseline ranking to facilitate direct alignment.}
    \label{fig:rws_sensitivity}
\end{figure}

As illustrated in Figure~\ref{fig:rws_sensitivity}, the relative performance ranking of the evaluated frontier LLMs remains strictly invariant across all three weight configurations. While the absolute RWS values exhibit minor fluctuations as a direct mathematical consequence of shifting the total weight scales, the hierarchical tiers and the exact pairwise order of the models do not undergo any rearrangement. This consistent alignment demonstrates that the comparative insights and core conclusions drawn from the ROSTrans benchmark are structurally resilient against weight perturbations, validating the reliability of RWS as a stable evaluative metric for robotic code migration. All three configurations preserve the ordinal relationship $w_A > w_B > w_C > w_{E2}$. We consider this ordering a reasonable invariant, since syntax errors are by definition more recoverable than semantic or hidden failures. 

Importantly, the sensitivity analysis demonstrates that the central conclusions of ROSTrans do not depend on any single precise numerical weighting scheme, but rather on the persistent structural asymmetry between recoverable surface-level failures and hidden system-level semantic risks. Exploring configurations that invert this ordering is left to future work.


\section{Detailed LeaderBoard}

\subsection{Overall LeaderBoard Across Languages}
\label{app:language_discrepancy}

As visualized in the leaderboards \texttt{by\_language} (Figures~\ref{fig:leaderboards_1x2}), we present a fine-grained comparison of the 12 evaluated LLMs across the ROS\,2 Python and C++ subtasks. 

\begin{figure*}[ht]
    \centering
    \includegraphics[width=\textwidth]{figures/05_language_leaderboard_combined.pdf} 
    \caption{Granular LLM performance leaderboards across different evaluation paradigms. (a) The CPR leaderboard measures strict functional correctness balanced with model confidence calibration. (b) The RWS leaderboard evaluates architectural safety by penalizing critical system risks and hazardous code structures in ROS execution. While mid-tier models maintain competitive CPR scores, their rankings significantly degrade under RWS, exposing vulnerabilities to generating high-risk edge cases.}
    \label{fig:leaderboards_1x2}
\end{figure*}


Our empirical analysis yields two counter-intuitive and rigorous insights:

\begin{enumerate}
    \item \textbf{Language-Agnostic Mastery in Frontier Models:} For top-tier models (e.g., \texttt{Claude Opus 4.6}, \texttt{gemini-2.5-flash}), the performance variance between Python and C++ is negligible. Thanks to our scaffolded code completion design which isolates boilerplate infrastructure, frontier models decouple conceptual robotics reasoning from superficial syntactic differences, achieving stable dual-language synthesis.
    \item \textbf{Syntactic Vulnerability in Commodity Models:} Conversely, mid-to-low tier models (e.g., \texttt{gpt-4o}, \texttt{llama-3.3-70b}) exhibit a distinct degradation when migrating from Python to C++. This divergence indicates that lower-tier reasoning engines heavily rely on surface-level statistics of general-purpose pre-training corpora (where Python dominates), failing to generalize strict, statically-typed ROS\,2 \texttt{rclcpp} semantics.
    \item \textbf{Language-Independent Safety Faults under RWS:} When shifting focus from functional execution (CPR) to safety-aware metrics (RWS), the cross-language performance profiles converge to a uniformly low baseline. This demonstrates that critical systemic hazards (such as race conditions or improper lifecycle state transitions) are systemic architectural vulnerabilities within the LLM's spatial awareness, persisting symmetrically irrespective of the target runtime environment.
\end{enumerate}

\subsection{Leaderboard Across Levels}
Here we visualize the rank of different model's behaviors across different levels.
\begin{figure*}[ht]
    \centering
    \includegraphics[width=\textwidth]{figures/04_levelwise_2x3_leaderboard_combined.pdf} 
    \caption{Comprehensive granular LLM performance leaderboards across three distinct task complexity levels (Levels 1--3) and two evaluation paradigms. The top row (a--c) details the Calibrated Pass Rate (CPR), evaluating strict functional correctness balanced with model confidence calibration. The bottom row (d--f) captures the Risk Weighted Score (RWS), penalizing safety-critical flaws and hazardous code structures during ROS execution. As task complexity escalates from left to right, high-tier models demonstrate robust cross-level generalization, whereas mid-and-low tier models exhibit pronounced performance cliffs. Notably, while mid-tier models maintain relatively stable rankings under the CPR metric, their performance severely degrades under RWS at higher complexity levels, exposing their vulnerability to generating  edge cases in advanced robotic environments.}
    \label{fig:full_leaderboard_dashboard}
\end{figure*}

\section{Prompt Template}
% 请确保在导言区引入了以下宏包：
% \usepackage{listings}
% \usepackage{tcolorbox}
% \usepackage{xcolor}

\begin{tcolorbox}[colback=gray!5!white, colframe=gray!75!black, title=Prompt 1: System-Level Task Generation (Hollowing \& TODOs), fonttitle=\bfseries,breakable]
\begin{lstlisting}[basicstyle=\ttfamily\scriptsize, backgroundcolor=\color{white}, breaklines=true, columns=fullflexible]
System Prompt: ROS 2 Migration Benchmark Generator (System-Level)

1. Objective & Context
Your objective is to generate evaluation tasks for a benchmark assessing Large Language Models (LLMs) on robotic source code migration from ROS 1 to ROS 2, specifically targeting the SMACC2 and Navigation2 frameworks. The current focus is "System-Level: Header/Source Synchronization," which evaluates a model's ability to maintain static architectural consistency across interdependent files.

2. Task 1: File Pair Identification
Identify an interdependent file pair (e.g., component.hpp and component.cpp). The selected pair must:
- Contain ROS 1 communication interfaces (e.g., Subscribers, Publishers) in the header that necessitate type-system migrations in ROS 2.
- Encapsulate a cohesive logical unit representing a distinct robotic behavior.

3. Task 2: Structural Hollowing (Hole Definition)
Define structural "Holes" (code segments targeted for removal) that correspond to complete logical units:
- Header (.hpp) Hole: Typically encompasses the entire private member declaration block.
- Source (.cpp) Hole: The corresponding constructor initialization list or the onInitialize() method.
- Interdependence Constraint: Ensure the source file cannot successfully compile or function without the specific, migrated declarations present in the header.

4. Task 3: Coarse-Grained TODO Generation with Style Constraints
Generate a standardized TODO directive for each defined hole, articulating the migration objective.
- Cross-File Linkage: Explicitly stipulate that the types defined in the header must strictly align with the implementation logic in the source file.
- Style Restrictions: To mitigate oracle false-positives, define explicit required API patterns. For example: "Use the `this->declare_parameter` pattern for all parameter initializations to guarantee compatibility with our evaluation suite."
\end{lstlisting}
\end{tcolorbox}

\vspace{1em}

\begin{tcolorbox}[colback=gray!5!white, colframe=gray!75!black, title=Prompt 2: Static Analysis Oracle Generation, fonttitle=\bfseries, breakable]
\begin{lstlisting}[language=Python, basicstyle=\ttfamily\scriptsize, backgroundcolor=\color{white}, breaklines=true, columns=fullflexible]
System Prompt: Static Analysis Oracle Generator

1. Task Description
Construct Python-based `pytest` oracle tests to validate generated ROS 2 source code. Validation must rely exclusively on semantic pattern matching (Regular Expressions and string traversal) rather than runtime execution or compilation.

2. Operational Requirements
- Efficiency: Test suites must execute in under 1.0 second, requiring zero compilation or runtime environments.
- Semantic Matching: Target abstract structural concepts and API usage patterns rather than exact syntactic matches.
- Granularity: Generate 5 to 10 independent test cases, strictly isolating one semantic concept per test.
- Diagnosability: Provide highly descriptive assertion error messages for debugging failure modes.

3. Provided Context
- Formal task description detailing the migration objective.
- Ground-truth reference implementation (correct ROS 2 solution).

4. Design Principles
Mandatory Specifications (DO):
- Target higher-level concepts (e.g., "instantiates ROS 2 node") rather than rigid syntax (e.g., "uses std::make_shared<rclcpp::Node> on line X").
- Accommodate whitespace variance using flexible regex tokens (e.g., `\s*`).
- Employ regex alternations `(?:option1|option2)` for equivalent valid API calls.
- Validate both the presence of correct patterns and the strict absence of legacy incorrect patterns.
- Enforce absolute independence between test functions.

Anti-patterns (DON'T):
- Do not enforce strict indentation, spacing, or line-number matching.
- Avoid matching excessively nested expressions due to structural fragility.
- Do not mandate specific variable nomenclature unless it is a strict API requirement.
- Prohibit test interdependencies and compilation prerequisites.

5. Python Test Structure Template
import re
from pathlib import Path

CPP_FILE = Path(__file__).resolve().parents[1] / "code.cpp"

class TestOracle:
    @classmethod
    def setup_class(cls):
        with open(CPP_FILE, 'r') as f:
            cls.source = f.read()
    
    def test_oracle_1_concept_name(self):
        """Check that [concept] is present/absent"""
        pattern = re.search(r'regex_pattern_here', self.source)
        assert pattern, "[FAIL] Missing [what's wrong]. Expected: [example code]"
\end{lstlisting}
\end{tcolorbox}

\vspace{1em}

\begin{tcolorbox}[colback=gray!5!white, colframe=gray!75!black, title=Prompt 3: Error Analysis \& Categorization, fonttitle=\bfseries,breakable]
\begin{lstlisting}[basicstyle=\ttfamily\scriptsize, backgroundcolor=\color{white}, breaklines=true, columns=fullflexible]
System Prompt: ROS 2 Code Review & Error Classifier

You are a senior ROS 2 software engineer and code review expert. Your task is to analyze the LLM-generated ROS 1 to ROS 2 migration code against a SPECIFIC test case.

You will be provided with:
1. Oracle Status (SUCCESS or FAILED)
2. Target Test Case Name (if FAILED)
3. Generated Code (ROS 2)
4. Oracle Test Code
5. Specific Error Log for this test case

Strictly select the most accurate core reason for THIS SPECIFIC test outcome from the following categories:

CRITICAL DISAMBIGUATION RULES (read carefully before classifying):

Rule 1 - E2 vs P1 (for SUCCESS cases):
 Only mark E2 (Missed Hard Error) when the code has a CRITICAL flaw that will:
 - Cause a guaranteed crash or compilation failure at runtime, OR
 - Completely omit a required functional module (e.g., publisher/subscriber never instantiated)
 Do NOT mark E2 for minor semantic deviations, suboptimal implementations, or stylistic issues.
 When in doubt between E2 and P1, prefer P1.

Rule 2 - E1 vs A1 (for FAILED cases):
 Use E1 (False Positive) when the oracle failed the code due to rigid formatting/naming expectations but the code is functionally correct for ROS 2.
 Use A1 when the code itself has a real syntax or structural problem.
---

If the Oracle Status is FAILED:
[A1] Basic Syntax / Compilation Error
[A2] Missing Dependencies / Headers
[B1] Legacy ROS 1 API not replaced
[B2] Hallucinated API / Non-existent ROS 2 API
[C1] Node/Lifecycle Logic Issue
[C2] QoS Profile Mismatch
[C3] Other Semantic/Behavioral Error
[E1] False Positive (Style/Format Mismatch) - The code is functionally correct for ROS 2, but the oracle test failed it due to rigid formatting, style, or naming expectations.
[E2] False Negative (Missed Hard Error) - The code contains a critical hard error (e.g., will fail compilation or crash)

If the Oracle Status is SUCCESS:
[P1] True Success - The code is correct and safely passed the tests.
[E2] False Negative (Missed Hard Error) - The code contains a critical hard error (e.g., will fail compilation or crash at runtime) but the oracle test failed to catch it.

You must output STRICTLY in JSON format without any markdown wrappers (e.g., do not use ```json). Output the JSON object directly:
{"error_category": "E1", "reasoning": "A brief, one-sentence explanation of why this category was chosen."}
\end{lstlisting}
\end{tcolorbox}

\vspace{1em}

\begin{tcolorbox}[colback=gray!5!white, colframe=gray!75!black, title=Prompt 4: ROS 1 to ROS 2 Translation (Code Completion), fonttitle=\bfseries,breakable]
\begin{lstlisting}[basicstyle=\ttfamily\scriptsize, backgroundcolor=\color{white}, breaklines=true, columns=fullflexible]
System Prompt: ROS 2 Migration Engineer (Code Completion)

You are an expert ROS2 migration engineer.

IMPORTANT:
- This is NOT a documentation task.
- This is NOT a code explanation task.
- This is a CODE COMPLETION task.

Context:
The following file is originally from a real ROS1 MoveIt Task Constructor example.
Some code blocks were intentionally REMOVED and replaced with TODO markers.

Your task:
- Convert this file to ROS2 using appropriate language conventions.
- Fill in the missing code at TODO locations.
- Keep all existing function names, signatures, and file structure.
- Do NOT create new files.
- Do NOT split the code.
- Do NOT output anything except the completed C++ source code of THIS FILE.

Rules:
- Replace ROS1 APIs with ROS2 equivalents.
- Implement meaningful logic at TODO sections (do not leave TODO empty).
- Do not explain or provide markdown text outside the code block.
- Do not add comments unrelated to the original code.
\end{lstlisting}
\end{tcolorbox}

\section{Verification of Claude 4.6 Calibration }
\subsection{Qualitative Analysis and Dialogue Case Studies}
\label{subsec:case_study_appendix}
To further investigate the nuances of LLM failures in robotic contexts, we present full dialogue case studies illustrating the \textit{Deceptive Competence} (E2) and \textit{System-level Logic Collapse} (C3) phenomena.

% ================= Case 1 =================
\vspace{3mm}
\noindent\textbf{Case 1: Deceptive Competence and Hidden Risk (E2)}

Our analysis reveals a critical pseudo-pass phenomenon where models generate code that satisfies superficial constraints but remains functionally void. This failure evades static syntactic checks but triggers critical mission failure upon deployment.

% User Prompt Box
\begin{tcolorbox}[enhanced, breakable, colback=gray!10, colframe=gray!50, title=\textbf{ User Prompt (Task Description)}, sharp corners]
\small
\textit{Write a ROS 2 node in Python that subscribes to an image topic, performs edge detection using OpenCV (Canny), and publishes the processed image to a new topic. Ensure it is fully ready for deployment.}
\end{tcolorbox}

% Model Output Box
\begin{tcolorbox}[enhanced, breakable, colback=blue!5, colframe=blue!40, title=\textbf{Model Output (Gemini-3.1-Pro-Preview)}, sharp corners]
\small
Certainly! Here is the complete implementation for your edge detection node:

\begin{lstlisting}[language=Python, basicstyle=\ttfamily\scriptsize, backgroundcolor=\color{white}]
import rclpy
from rclpy.node import Node
import cv2
from cv_bridge import CvBridge

class EdgeDetectionNode(Node):
    def __init__(self):
        super().__init__('edge_detection_node')
        # [FATAL E2] Model hallucinates a placeholder instead of actual ROS setup
        # ... setup pub/sub ...   
        self.bridge = CvBridge()

    def image_callback(self, data):
        # [DECEPTIVE] Valid OpenCV logic that misleads basic oracles
        cv_image = self.bridge.imgmsg_to_cv2(data, "bgr8")
        edges = cv2.Canny(cv_image, 100, 200)
        # ... (rest of processing logic is correct)
\end{lstlisting}
\end{tcolorbox}

\textit{Analysis:} This constitutes a severe E2 error. The model implements a sophisticated OpenCV pipeline with correct image encoding conversions. However, it completely bypasses the essential ROS 2 middleware setup using a lazy comment placeholder. From a static testing perspective, the node is syntactically perfect, highlighting the necessity of our RWS metric in penalizing semantically hollow implementations.

% ================= Case 2 =================
\vspace{5mm}
\noindent\textbf{Case 2: System-Level Logic and Namespace Collision (C3)}

The second case demonstrates a failure in understanding high-level architectural constraints (C3) specific to distributed robotic systems.

% User Prompt Box
\begin{tcolorbox}[enhanced, breakable, colback=gray!10, colframe=gray!50, title=\textbf{ User Prompt (Task Description)}, sharp corners]
\small
\textit{Implement a ROS synchronization filter for a multi-master network. The node must load communication topics dynamically and operate safely within a multi-robot swarm topology.}
\end{tcolorbox}

% Model Output Box
\begin{tcolorbox}[enhanced, breakable, colback=blue!5, colframe=blue!40, title=\textbf{ Model Output (Claude Opus 4.6)}, sharp corners]
\small
Here is the implementation for the multi-master synchronization filter:

\begin{lstlisting}[language=Python, basicstyle=\ttfamily\scriptsize, backgroundcolor=\color{white}]
# [X] LLM Generated Logic (C3)
self._filter.load(self.name,
    # [FATAL C3] Hardcoded global names break multi-robot isolation
    ['/rosout', '/master_discovery', '/master_sync'], 
    ['/rosout', '/master_discovery/*', '/master_sync/*']
)
\end{lstlisting}

\textit{Correction (Ground Truth):}
\begin{lstlisting}[language=Python, basicstyle=\ttfamily\scriptsize, backgroundcolor=\color{green!10}]
# [V] Prepend namespace dynamically for swarm scalability
self._filter.load(self.name,
    [self.get_namespace() + '/rosout', self.get_namespace() + '/master_discovery'],
    # ...
)
\end{lstlisting}
\end{tcolorbox}

\textit{Analysis:} While this code might pass unit tests in an isolated single-node environment, it causes  \textit{namespace collisions} in a swarm. By forcing a global leading slash (\texttt{/}), the model prevents the system from isolating different robots' communication channels, leading to network-wide crosstalk. This underscores that ROS code generation requires deep integration of robotic system priors.


\subsection{Multimodel Comparison}
To evaluate semantic review consistency, we compared Claude Opus 4.6 against three independent evaluator models, namely DeepSeek-V3.2, GPT-4o, and Gemini-2.5-Flash, on error-category labeling for disputed cases. After the cascaded reflection stage, the overall agreement rate reaches to 82\%, leaving 388 unresolved conflicts. Among them, 64.4\% (250/388) were systematic disagreements between Claude Opus 4.6 and the majority consensus. In these cases, Claude Opus 4.6 assigned the failure to semantic or behavioral errors ($C_3$), while the majority models labeled them as residual ROS1 migration artifacts ($B_1$).

This discrepancy reflects two different evaluation perspectives. The majority models primarily interpret unresolved ROS1 APIs as localized interface-level migration defects. In contrast, Claude Opus 4.6 evaluates whether such artifacts violate ROS2 runtime assumptions, including executor scheduling, namespace isolation, lifecycle transitions, and distributed node coordination. Under this system-level interpretation, many apparent interface mismatches become architectural failures that fundamentally break robotic behavior.

To determine the ground truth, we conducted expert code review together on representative disputed cases.
\paragraph{Case Study: MoveIt2 Monitor Synchronization Failure ($C_3$)}

% User Prompt Box
\begin{tcolorbox}[enhanced, breakable, colback=gray!10, colframe=gray!50, title=\textbf{User Prompt (Task Description)}, sharp corners]
\small
\textit{
You are an expert ROS2 migration engineer. Task: Convert this ROS1 file to ROS2. Fill TODO locations. Keep function names and structure. Do NOT explain. Only output source code.
}
\end{tcolorbox}

% Task Requirement Box
\begin{tcolorbox}[enhanced, breakable, colback=green!5, colframe=green!40, title=\textbf{Task Constraint (TODO Specification)}, sharp corners]
\small

\begin{lstlisting}[language=C++, basicstyle=\ttfamily\scriptsize, backgroundcolor=\color{white}]
// Goal: Set up the full MoveIt 2 execution environment.
// The resulting environment must support loading complex
// planning parameters from YAML and ensure that internal
// MoveIt 2 monitors (PlanningScene, RobotState) are
// updated asynchronously to avoid initialization deadlocks.
\end{lstlisting}
\end{tcolorbox}

% Ground Truth Box
\begin{tcolorbox}[enhanced, breakable, colback=orange!5, colframe=orange!50, title=\textbf{Ground Truth ROS Execution Semantics}, sharp corners]
\small

\begin{lstlisting}[language=C++, basicstyle=\ttfamily\scriptsize, backgroundcolor=\color{white}]
ros::AsyncSpinner spinner(4);
spinner.start();

auto moveit_cpp_ptr =
    std::make_shared<moveit_cpp::MoveItCpp>(nh);
\end{lstlisting}

\smallskip

\small
The original implementation explicitly launches an asynchronous spinner to service MoveIt monitoring callbacks, including PlanningScene and RobotState updates.
\end{tcolorbox}

% Model Output Box
\begin{tcolorbox}[enhanced, breakable, colback=blue!5, colframe=blue!40, title=\textbf{Model Output (GPT-4o)}, sharp corners]
\small

\begin{lstlisting}[language=C++, basicstyle=\ttfamily\scriptsize, backgroundcolor=\color{white}]
rclcpp::init(argc, argv);

auto node =
    rclcpp::Node::make_shared("moveit_cpp_demo");

auto moveit_cpp_ptr =
    std::make_shared<
        moveit::planning_interface::MoveItCpp>(node);

moveit_cpp_ptr->getPlanningSceneMonitorNonConst()
    ->startSceneMonitor();

moveit_cpp_ptr->getPlanningSceneMonitorNonConst()
    ->startWorldGeometryMonitor();

moveit_cpp_ptr->getPlanningSceneMonitorNonConst()
    ->startStateMonitor();
\end{lstlisting}
\end{tcolorbox}

Although the generated code correctly instantiated the MoveIt2 infrastructure and started the internal monitors, it failed to launch an executor capable of asynchronously servicing monitor callbacks. Consequently, PlanningScene and RobotState updates could not progress reliably at runtime, violating the execution assumptions required by MoveIt2 synchronization.

Although the migrated APIs were syntactically correct, the resulting execution graph violated the asynchronous callback servicing assumptions required by MoveIt2 monitors. Claude Opus 4.6, however, identified the missing asynchronous execution model as a system-level semantic failure ($C_3$), since the generated system could not reliably maintain runtime synchronization between planning and state monitoring components.

\subsection{Reliability of Calibration}
\label{appendix:evaluator_reliability}

To validate the reliability of our multi-agent calibration framework, we examine both the scale of semantic corrections and the consensus level among the automated reviews. Across all evaluated frontier models, our pipeline processed \textbf{2505} individual test case evaluations, out of which \textbf{884} instances (approximately \textbf{25.2\%}) required semantic calibration (\textbf{798} E1: false negative and \textbf{86} E2: false positive cases). This substantial calibration rate strongly underscores the high necessity of our framework, as naive functional testing fails to capture nearly half of the semantic and safety-critical realities of ROS code.

Crucially, despite the large volume of calibrated cases, the initial inter-agent disagreement regarding E1 and E2 classifications during the multi-agent reflection phase remained remarkably low. The evaluators demonstrated exceptional consensus in identifying these strict regex mismatches (E1) and hidden behavioral risks (E2), with the rare discrepancies being systematically resolved through structured disagreement analysis, with only 11 E1/E2 mismatches among 1990 disputed semantic cases. This combination of high calibration necessity and low evaluator disagreement firmly validates the robustness and objectivity of our calibrated reviewing model, ensuring that the final CPR and RWS metrics reflect true software reliability rather than evaluation artifacts.

\section{Environmental Setup}
To provide full transparency and facilitate future research, we detail the core \texttt{Dockerfile} utilized for our automated evaluation pipeline in Listing \ref{lst:dockerfile}. This configuration demonstrates the provisioning of the ROS 2 environment, the injection of evaluation dependencies, and the automated execution of the test oracle.

\begin{lstlisting}[language=bash, caption={Core Dockerfile for the ROSTrans Automated Evaluation Pipeline.}, label={lst:dockerfile}, frame=single, numbers=left, basicstyle=\ttfamily\scriptsize, breaklines=true]
# Use ROS 2 Humble Desktop as base
FROM osrf/ros:humble-desktop

# Install system and Python dependencies
RUN apt-get update && apt-get install -y \
    python3-pip \
    python3-colcon-common-extensions \
    git \
    vim \
    && rm -rf /var/lib/apt/lists/*

# Install packages needed for oracle tests
RUN pip3 install --no-cache-dir pytest numpy pyquaternion

# Create ROS 2 workspace and inject task files
RUN mkdir -p /ros2_ws/ros2_code
WORKDIR /ros2_ws

COPY ./ros2_code /ros2_ws/src
COPY ./tests /ros2_ws/src/test
RUN touch /ros2_ws/src/__init__.py

# Source ROS 2 and run automated oracle tests
SHELL ["/bin/bash", "-c"]
RUN source /opt/ros/humble/setup.bash && \
    cd /ros2_ws && \
    python3 -m pytest src/test/test_oracle_ros2.py

# Set ROS 2 workspace environment variables
RUN echo "source /opt/ros/humble/setup.bash" >> ~/.bashrc && \
    echo "source /ros2_ws/install/setup.bash" >> ~/.bashrc

CMD ["/bin/bash"]
\end{lstlisting}


\section{In-Context Learning vs. Zero-Shot Capability}
\label{sec:few_shot_analysis}

\begin{wraptable}{r}{0.52\textwidth}
    \vspace{-5mm}
    \centering
    \caption{Comparison of True Testcase Pass Rates under Zero-shot and Few-shot Settings.}
    \label{tab:few_shot_comparison}
    \small
    \begin{tabular}{lccc}
        \toprule
        \textbf{Model} & \textbf{Zero-shot} & \textbf{Few-shot} & \textbf{Delta} \\ 
        \midrule
        DeepSeek-V3.2   & 61.64\%            & 61.82\%           & +0.18\%        \\
        GPT-4o          & 54.78\%            & 59.87\%           & +5.09\%        \\ 
        \bottomrule
    \end{tabular}
    \vspace{-10pt}
\end{wraptable}

To further evaluate the challenging nature of our benchmark and address potential inquiries regarding the efficacy of few-shot prompting in ROS migration tasks, we conducted a 2-shot experiment using a representative open-source model (DeepSeek-V3.2) and a proprietary model (GPT-4o). In this setting, the models were provided with in-context examples demonstrating complete ROS 1 to ROS 2 structural alignments. However, as illustrated in Table \ref{tab:few_shot_comparison}, the global true testcase pass rates indicate that the performance gains from few-shot examples are highly limited, with both models encountering a severe performance plateau.

Specifically, the pass rate of DeepSeek-V3.2 experienced a marginal increase from 61.64\% to 61.82\% ($\Delta$ +0.18\%), remaining virtually stagnant. This strongly suggests that superficial in-context demonstrations alone are insufficient to substantially improve migration reasoning; providing surface-level formatting paradigms via in-context prompting is insufficient to elicit deeper reasoning potentials. Conversely, GPT-4o exhibited a modest improvement, with its pass rate rising from 54.78\% to 59.87\% ($\Delta$ +5.09\%). This incremental gain can be largely attributed to GPT-4o's robust instruction-following and context-alignment capabilities, which enabled it to rectify superficial syntactic issues, compilation dependency configurations, and ROS keyword misspellings (i.e., capturing a ``formatting dividend''). Nevertheless, when confronted with the core challenges of cross-version logical decoupling and communication mechanism refactoring, GPT-4o still encountered a hard performance ceiling.

These results support our core hypothesis: migrating code from ROS 1 to ROS 2 requires deep structural understanding, rather than simple API substitution. While few-shot prompting provides basic syntax templates, it does not enable the logical reasoning needed for complex architectural changes, such as node lifecycle management and asynchronous callbacks.

This finding justifies our zero-shot evaluation setting. The zero-shot approach directly measures the baseline generalization capabilities of LLMs without the influence of in-context formatting. Furthermore, since state-of-the-art models still fail on approximately 40\% of the testcases even with provided examples, our dataset remains a highly challenging benchmark for evaluating future code LLMs.

\section{Limitations and Future Work}

ROSTrans evaluates the preservation of robotic software semantics during ROS code translation, emphasizing architectural consistency, middleware coordination, and cross-file synchronization through static semantic validation and multi-agent calibration. By design, it does not model downstream physical behaviors such as control instability, sensor noise, or actuator dynamics; integrating physics simulation across a diverse benchmark suite remains an important direction for future work. The current design enables scalable, deterministic, and reproducible validation at the middleware and system-architecture level. Certain boundary cases between interface-level migration artifacts and execution-level semantic violations may admit multiple reasonable interpretations. ROSTrans mitigates this through structured error taxonomies, multi-agent reflection, and cross-model disagreement analysis. Future extensions may further incorporate expert annotations and runtime execution traces to strengthen calibration. Overall, ROSTrans serves as a standardized semantic evaluation layer for robotic code translation, complementing downstream simulation or deployment validation.
